# Supplementary material for: Real space observation of magnon interaction with driven space-time crystals
Source: arXiv:1911.13192 source file (2019-11-29)
Supplement: Supplementary file 1 [file Supplemental_Material.pdf]

# Micromagnetic simulations

To validate and understand experimental results micromagnetic simulations with the use of MuMax3 [1] have been performed. In simulations, a 30 nm thick magnetic stripe of the lateral dimensions 11 µm and 1.4 µm characterized by the magnetic properties $A_{ex}$=13 pJ/m, $M_S$=700 kA/m, and damping $\alpha$=0.008 has been considered. This system has been discretized by the unit cells of lateral dimensions equal 5×5 nm$^2$ being smaller than the exchange length $l_{\text{ex}} = \sqrt{2A/(\mu_0 M_S^2)} \approx 6.5$ nm and one unit cell across the thickness (30 nm). In all simulations, the field of value 8 mT aligned along the stripe's axis (the *x*-axis) has been applied.

The simulations, firstly, has been used to calculate a static magnetic configuration, which, secondly, has been perturbed by the microwave magnetic field (mf). The scheme of the excitation determines the type of obtained spectral response. Therefore, in order to calculate spin wave (SW) dispersion relation a broadband point source-like excitation was used in the form

$$\mathbf{h}_{\text{mf}}(\text{r}, \text{t}) \propto \text{sinc}(k_{\text{cut}} r)\text{sinc}(2\pi f_{\text{cut}} t)\hat{\boldsymbol{e}}_y,$$

where $r$ denotes the distance from the center of the stripe, $f_{cut}$ and $k_{cut}$ are the cut-off frequency and wavenumbers, respectively, defining the maximal value of the frequency and wavevector being excited. Similarly, in order to verify the spectral response of the system on a harmonic, spatially uniform mf of various amplitudes the mf profile $\mathbf{h}_{\text{mf}}(\text{r}, \text{t}) = h_{\text{mf}}\text{sin}(2\pi f t)\hat{\boldsymbol{e}}_y$ (where $h_{\text{mf}}$ and $f$ denotes the amplitude and frequency of the mf) has been assumed. The spectral response (in the first case spin wave dispersion relation) was then computed by transforming the time-dependent magnetization into the frequency and wavevector space using two dimensional fast Fourier transformation (FFT).

# Spin waves dispersion relation

Simulated spin wave dispersion relation is displayed in Figure S1. The dispersion relation exhibits a dense spin wave spectrum with multiple magnonic bands corresponding to subsequent spin wave modes with different quantization across the stripe's width. Interestingly, there are no solutions available for SWs of wavelengths shorter than ca. 260 nm for the frequency 4.2 GHz, although it was observed experimentally. It is important to remind here, that the dispersion relation has been obtained only for the linear SW excitations by an application of low power point-source-like spin wave source, therefore, any phenomena related to the non-linear nature of spin waves are not caught in that picture. The analytically derived dispersion for the first three bands has been calculated according to Ref. [2] combined with the effective boundary conditions for a magnetic stripe derived by Guslienko et al. [3].

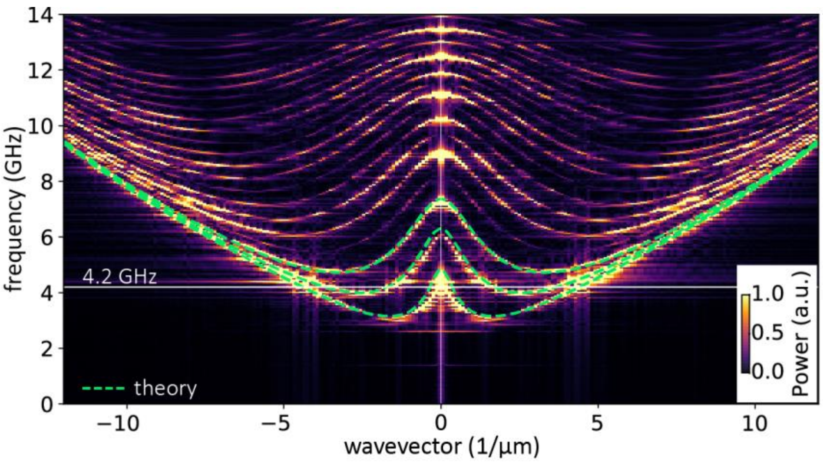


Figure S1. SW dispersion relation. Color brightness correspond to the intensity of SWs of a given frequency and wavevector. Bright, green line corresponds to the dispersion of the backward volume mode in the uniform thin film. Perfect match between results of a finite Py stripe and infinite thin film is achieved for longer wavevectors. The horizontal white line distinguishes SWs of the frequency 4.2 GHz.

## Spectral response on spatially uniform harmonic excitation of various amplitudes

In order to verify whether the non-linearity is responsible for the emergence of the new larger $k$-vector mode, the influence of the amplitude of the spatially uniform mf on spin wave spectra is studied. The simulations are performed for a harmonic spatially uniform SWs excitation of various frequencies in the range of 4.0-4.8 GHz. The analysis of these results is presented in Figure S2. The spectra (shown in lower panels) combined with the corresponding averaged in time $x$-components of magnetization (shown in upper panels) are depicted only for the selected simulations for various field amplitudes and frequencies. The results for the frequency 4.2 GHz are displayed in Figure S2(a-d), whereas, results for two frequencies 4.5 GHz (just below the frequency of the uniform precession mode, FMR) and 4.6 GHz (just above FMR) are shown in Figure S2(e-f) and (g), respectively. Keep in mind that since the amplitudes of the mf are high, the frequency of the uniform precession mode depends on the amplitude of the mf. In our system, the FMR frequency for the linear excitations is equal to 4.9 GHz, but the induced non-linearity causes a downshift of the FMR frequency.

It is visible that for small values of $h_{\mathrm{mf}}$ (Figure S2(a)) , there are excited only SWs of the frequency 4.2 GHz corresponding to all the modes present in the dispersion for that frequency (Figure S1). However, while $h_{\mathrm{mf}}$ increases, the modes of the doubled frequency of the microwave antenna appear (Figure S2(b-c) and (e-f)). For instance, there are visible excitations of wavelength 95 nm ($k$=10.5 μm$^{-1}$) which are not detected experimentally though. Above some amplitude of $h_{\mathrm{mf}}$ the spectra become very noisy (Figure S2(d)) what is related to the demagnetization of the stripe.

However, the most interesting observation is the case presented in Figure S2(c) for mf amplitudes of 450 μT and a frequency of 4.2 GHz. An additional bright spot corresponding to the frequency of the applied mf (4.2 GHz) and much shorter wavelengths (ca. 130 nm corresponding to $k\approx$7.7 μm$^{-1}$) appears in the spectra. This one is observed experimentally. Interestingly, this excitation is not present in the previously obtained SW dispersion relation for the uniformly magnetized thin film. It is noteworthy that we haven't been able to find this mode for lower damping values (e.g. $\alpha$=10$^{-4}$) what means that the appearance of this mode is related to some specific relation of the mf amplitude with SW damping. Additional simulations for 4.5 GHz being just below FMR frequency shows that this new mode is also visible for $h_{\mathrm{mf}}$=300 μT whereas for 4.6 GHz (just above FMR) this

mode doesn’t appear even for $h_{\mathrm{mf}}$=450 μT. It may suggest that the appearance of this mode is related not only to the amplitude of the mf, but also the frequency, and it is the most efficient for frequencies near FMR frequency, but not exceeding it.

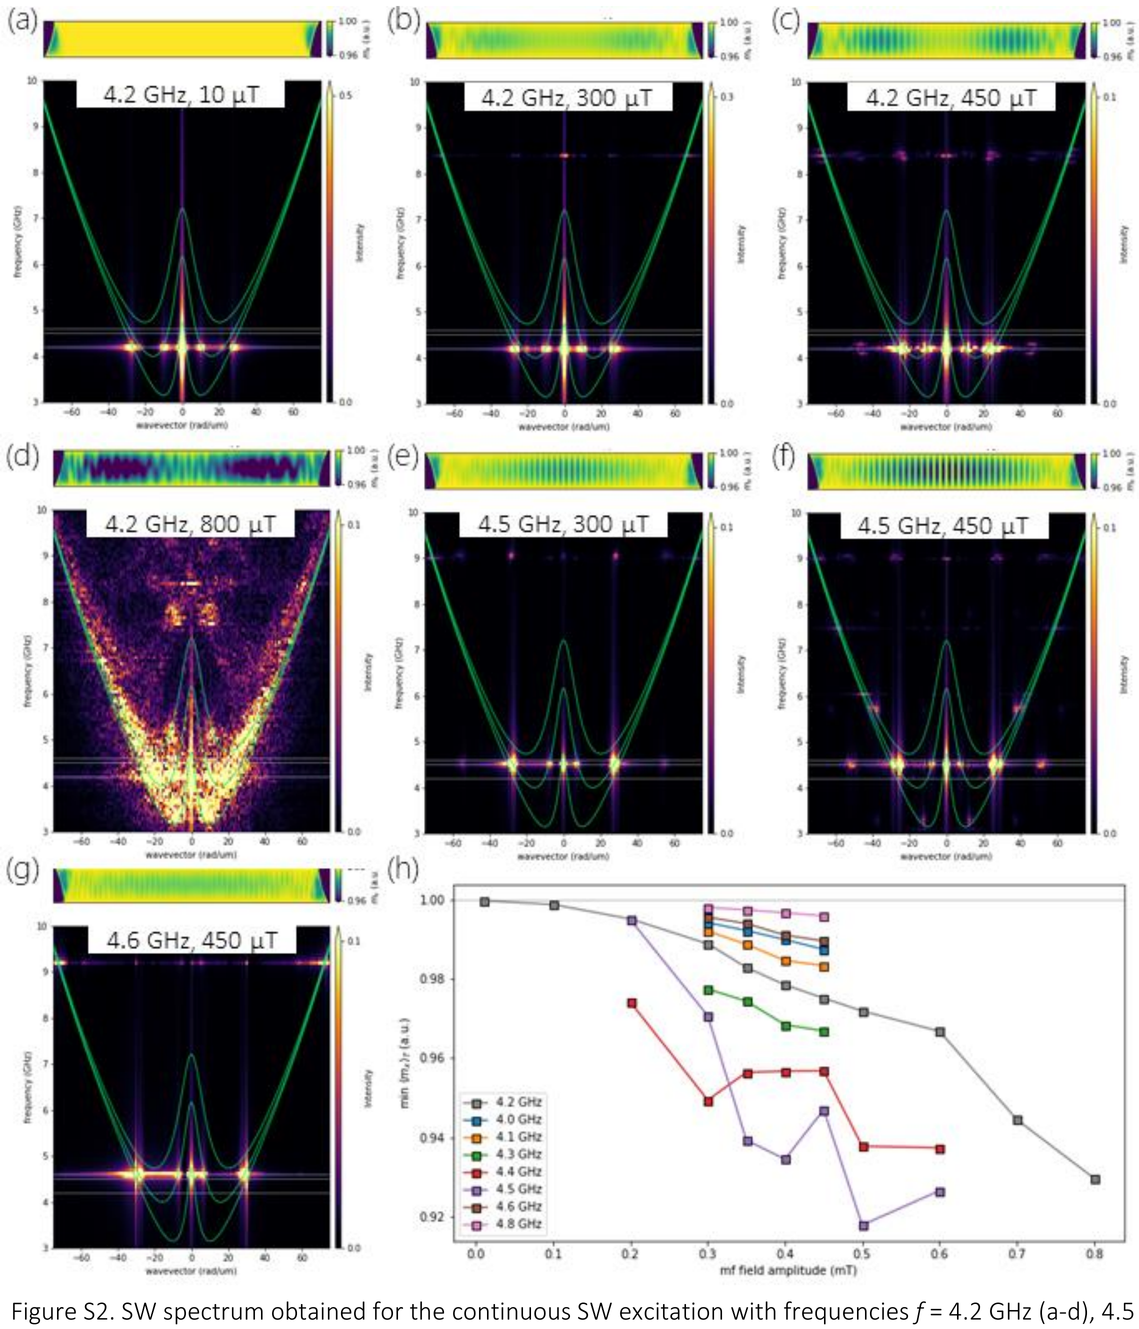


Figure S2. SW spectrum obtained for the continuous SW excitation with frequencies $f$ = 4.2 GHz (a-d), 4.5 GHz (e-f) and 4.6 GHz (g) and for different amplitudes of in-plane microwave field are visible in lower panels whereas the averaged in time x-component of magnetization for corresponding scenarios are shown in the upper panels. (h) The maximal angles of magnetization precession calculated in the central stripe’s part calculated for different frequencies and amplitudes of the exciting fields.

# Periodic structure of periodic dynamic magnetization domains

The existence of an additional mode being located in the spin wave spectrum far outside the spin wave dispersion of the uniformly magnetizes stripe suggests that for this particular case, SWs do not longer propagate in the uniformly magnetized stripe, precisely, the central part of the stripe is no longer uniformly magnetized.

Indeed, results of simulations show that for some range of $h_{\mathrm{mf}}$ where additional mode appears, the averaged in time *x*-component of magnetization[1] is no longer uniformly aligned along the *x*-axis (see the upper panels in Figure S2). It is visible that its value is periodically decreasing, which suggests that these periodic nonuniformities serve as scattering centers, like in the case of magnonic crystals.

To better visualize that, let us show the in-plane [$\Theta_{\mathrm{IP}} = \arcsin(m_y)$] and out-of-plane [$\Theta_{\mathrm{OOP}} = \arcsin(m_z)$] deviations of the magnetization vector from the *x*-axis in dependence on time and *x*-coordinate for a crossection along the stripe's center (at $y$=0.7 µm) obtained for $h_{\mathrm{mf}}$=450 µT and 4.2 GHz presented in Figures S3(a) and (b), respectively.

We see a periodic-like modulation of the magnetization vector in both time and space. There are present nodes for which $m_x$=1, and between these nodes magnetization oscillates. However, unlike in the case of a typical standing wave [$m \propto A\cos(kx)\sin(2\pi f)$], all these oscillations are in-phase. Phenemologically it could be described as

$$m_x \propto \left(1 - A\cos^2\left(\frac{2\pi}{a}x\right)\right)\sin(2\pi f)$$

where *A* is the amplitude of these oscillations and *a* is the period of the emerged domain pattern. According to simulations, this period is equal to the wavelength of the fundamental mode with positive group velocity (ca. 260 nm) and *a* is two times longer than the wavelength of this new short-wavelength mode. It is also visible, that these oscillations are characterized by strong in-plane ellipticity, the angles for the in-plane projection of magnetization are ca. 5 times larger than for the out-of-plane projection.

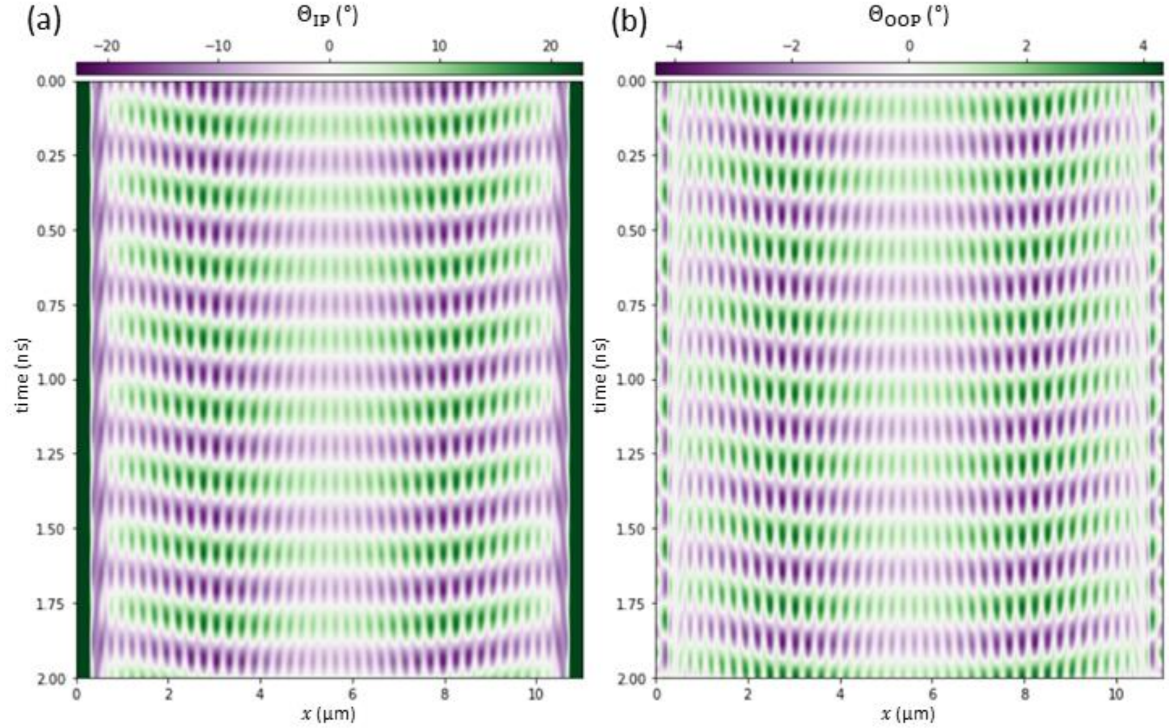


Figure S3. SW spectrum obtained for the continuous SW excitation by a single frequency *f* = 4.2 GHz and different amplitudes of the in-plane microwave field. Color brightness corresponds to normalized SW intensity (100% corresponds to the maximal amplitude for *f* = 4.2 GHz).

[1] $\langle m_x \rangle = \int_t^{t+2/f} m_x(t,x)dt$

It seems that we can observe the creation of a periodic magnetization domain pattern with periodically arranged "dynamic" and "static" domains with the amplitude of magnetization oscillations in these "dynamic" domains depending on both the amplitude and frequency of the mf. It is presented in Figure S2(h) where the dependence of the amplitude of the oscillations of these "dynamic" domains on mf amplitude for different frequencies is shown. We find that a larger amplitude of the mf leads to a larger amplitude of these oscillations. It is also visible, that the amplitude of these oscillations increases while the frequency is approaching FMR frequency and drastically decreases when the frequency exceeds the FMR frequency (4.6 and 4.8 GHz). The nonmonotonic dependence for 4.4 and 4.5 GHz results from the dependence of the non-linear FMR on the mf amplitude.

To further confirm, that we do not have a typical standing wave of high amplitude, let us analyze the process of its formation. Figure S4 shows the angle of in-plane oscillations of the magnetization in dependence on time (vertical axis) and *x*-coordinate (horizontal axis). It is visible that this "dynamic" magnetization pattern nucleates at the 90° Neel domain walls (present at shorter sides of the stripe) from where it is extending towards the stripe's center. For the frequency 4.2 GHz it needs ca. 14 ns until the steady-state is reached. In the case of a standing wave, we would expect two waves propagating from the sides and then interfere creating a standing wave.

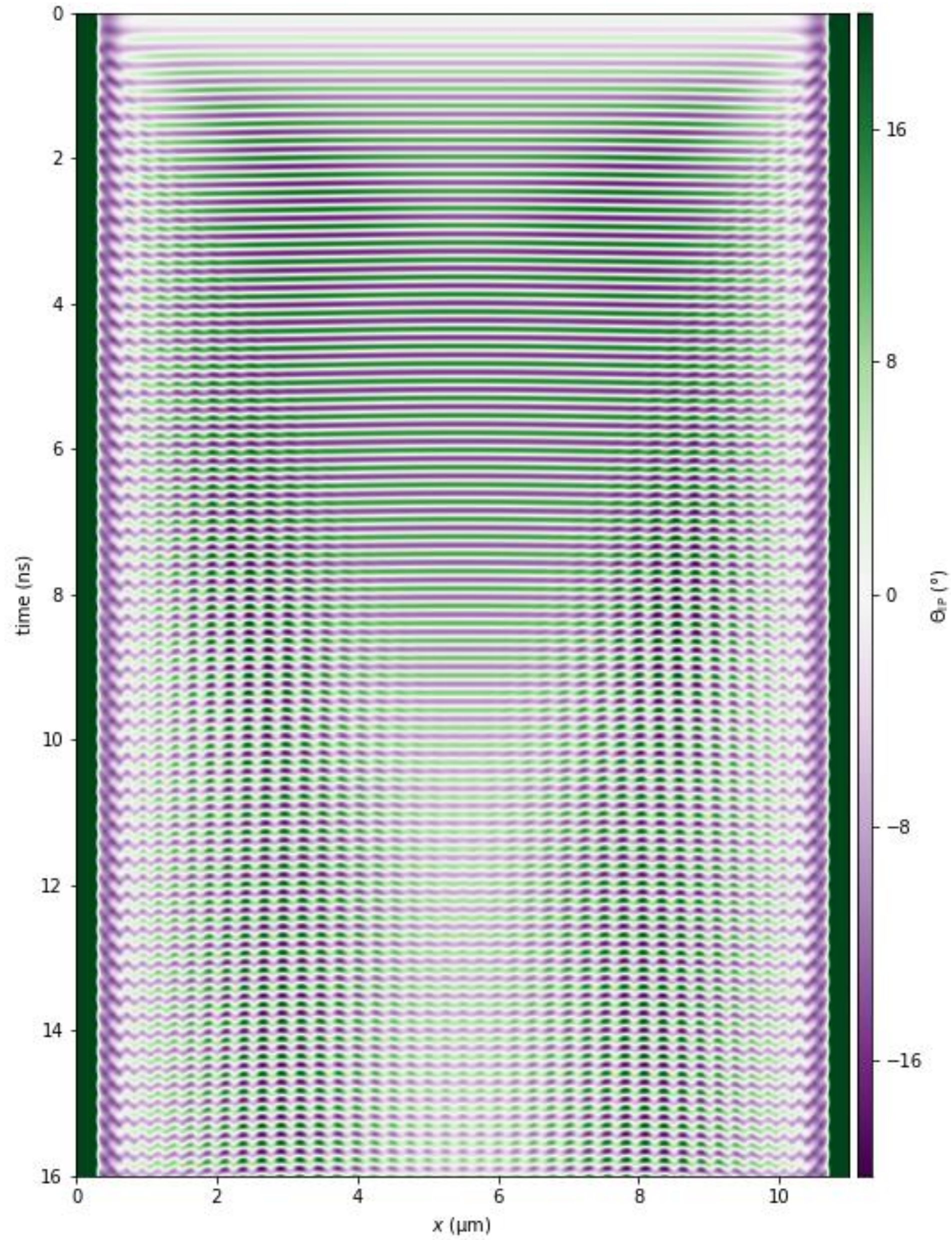


Figure S4. The dependence of the in-plane angle of magnetization vs. time and $x$-coordinate showing the formation of periodic in time and space magnetization domain pattern.

## Simplified system

To cut down the situation, let us analyze a simplified model. We consider a 200 nm wide and 30 nm thick infinitely long Py stripe with the following magnetic parameters: $M_S$=650 kA/m and $A_{ex}$=13 pJ/m. For that stripe, the SW spectrum is much sparser than for the wider stripe. That is, there is a visible larger separation between subsequent magnonic bands. Importantly, for the considered case, the frequency of the bottom of the second band is greater than the FMR frequency. Moreover, due to decreased stripe's width, the FMR frequency is shifted towards higher frequencies, *i.e.*, 8.7 GHz. Let us consider SW excitation by the mf of amplitude 1.2 mT and frequency 8.3 GHz that is (a) spatially uniform and (b) spatially uniform with one defect introduced in the central part of the simulated system for $|x|$<8 nm, where $h_{\mathrm{mf}} = 0$, see Figure S5(a). Now, we discuss how these fields influence the static magnetization configuration by looking at the time-averaged (over two periods of the driving field) $m_x$ magnetization components (along the stripe axis), *i.e.*, $\langle m_x \rangle = \int_t^{t+2/f} m_x(t,x)dt$ (see Figure S5(b-d)). It is displayed that for the first case with the ideall y uniform magnetic field, the averaged in time magnetization

is spatially uniform (see black dashed line). On the contrary, for the second case with this small nonuniformity of the driving field at $x$=0, in the central part of the stripe is formed a periodical magnetization pattern expanding both leftwards and rightwards while the driving field is applied. Nodes of that magnetization pattern are related to regions where $<m_x>$=1 are stationary (not moving in time) whereas the regions with non-unity $<m_x>$ are related to the dynamic magnetization domains where magnetization oscillates everywhere in-phase (not shown in Figure S5), similarly like in the previous case for the wider stripe shown in Figure S4. Interestingly, the velocity of the expansion of this dynamic magnetization pattern is ca. 400 m/s, where the phase velocity of SWs for the same frequency is ca. 750 m/s.

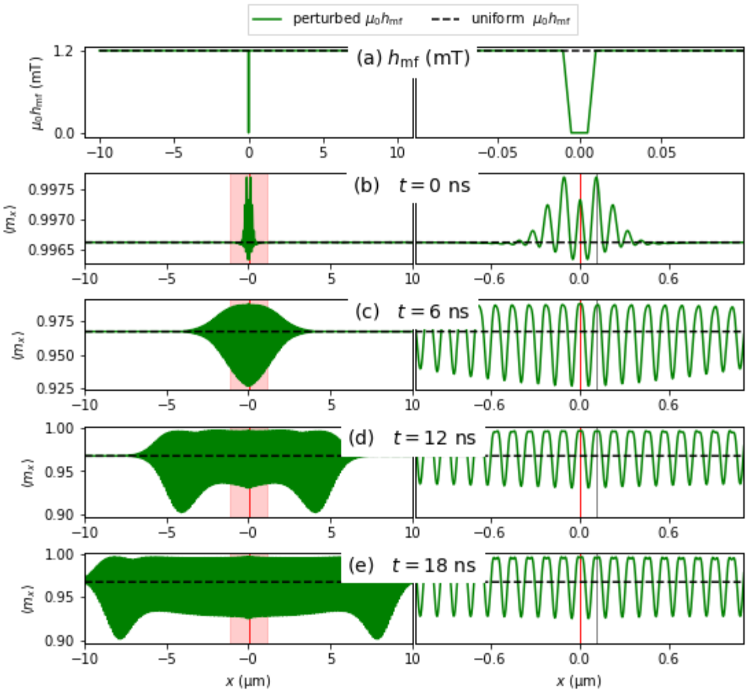


Figure S5. Results of simulations performed for 200 nm narrow, infinite waveguide excited by the harmonic microwave field of frequency $f$=8.3 GHz being just below FMR frequency (8.7 GHz). (a) Profile of the microwave field along the $x$-axis. On the right hand side is a visible zoomed-in central region. (b)-(d) Averaged for one period of time $m_x$ component of the magnetization for different times. On the right-hand sides there are visible zoomed-in regions highlighted by the red color on left panels. The solid green line corresponds to the case with perturbed $h_{\mathrm{mf}}(x)$ whereas dashed black line to the uniform $h_{\mathrm{mf}}(x) = \mathrm{const.} = 1.2$ mT.

## Literature


[1] A. Vansteenkiste, J. Leliaert, M. Dvornik, M. Helsen, F. Garcia-Sanchez, and B. Van Waeyenberge, *The design and verification of MuMax3*. AIP advances, 4(10), 107133 (2014).

[2] B. A. Kalinikos and A. N. Slavin, *Theory of dipole-exchange spin wave spectrum for ferromagnetic films with mixed exchange boundary conditions.* Journal of Physics C: Solid State Physics **19**, 7013 (1986)

[3] K. Yu. Guslienko, S. O. Demokritov, B. Hillebrands, and A. N. Slavin. *Effective dipolar boundary conditions for dynamic magnetization in thin magnetic stripes.* Phys. Rev. B **66**, 132402 (2002).
